# Supplementary material for: Distributed Random Reshuffling over Networks
Source: arXiv:2112.15287 source file (2023-03-23)
Supplement: Supplementary file 1 [file TSP_Final_supp.pdf]

## SUPPLEMENTARY MATERIAL

## APPENDIX B

## PARTS OF PROOFS FOR STRONGLY CONVEX CASE

## A. Proof of Lemma 1

*Proof.* Based on Assumption 1, we have

$$\begin{aligned}\|W\omega - \mathbf{1}\bar{\omega}^\top\| &= \left\| \left( W - \frac{1}{n}\mathbf{1}\mathbf{1}^\top \right) (\omega - \mathbf{1}\bar{\omega}^\top) \right\| \\ &\leq \left\| W - \frac{1}{n}\mathbf{1}\mathbf{1}^\top \right\| \left\| (I - \frac{1}{n}\mathbf{1}\mathbf{1}^\top)\omega \right\|.\end{aligned}$$

□

## B. Proof of Lemma 6

*Proof.* Using (5) and (7), it follows

$$\begin{aligned}\mathbb{E}[D_{\bar{s}_\ell}(\bar{x}_*, x^*)] &\leq \frac{L}{2} \mathbb{E}[\|\bar{x}_*^\ell - x^*\|^2] \\ &= \frac{L\alpha_t^2}{2} \mathbb{E} \left[ \left\| \sum_{k=0}^{\ell-1} \left( \frac{1}{n} \sum_{i=1}^n \nabla f_{i, \pi_k^i}(x^*) \right) \right\|^2 \right] \\ &\leq \frac{L\alpha_t^2}{2n} \sum_{i=1}^n \mathbb{E} \left[ \left\| \sum_{k=0}^{\ell-1} \nabla f_{i, \pi_k^i}(x^*) \right\|^2 \right] \\ &= \frac{L\alpha_t^2}{2n} \sum_{i=1}^n \frac{\ell(m-\ell)}{(m-1)m} \sum_{j=1}^m \|\nabla f_{i,j}(x^*)\|^2 \leq \frac{L\alpha_t^2 m}{4} \sigma_*^2, \quad (44)\end{aligned}$$

where (44) holds according to Proposition 1 in [23]. The lower bound can be derived similarly. □

## C. Proof of Lemma 9

*Proof.* Unroll (16) in Lemma 8 and invoke the relation between  $\sigma_{\text{shuffle}}^2$  and  $\sigma_*^2$  according to Lemma 6, we get

$$\begin{aligned}H_t &\leq \prod_{j=0}^{t-1} \left( 1 - \frac{\alpha_j \mu}{4} \right)^m H_0 + \sigma_*^2 \sum_{j=0}^{t-1} \left\{ \left[ \prod_{q=j+1}^{t-1} \left( 1 - \frac{\alpha_q \mu}{4} \right)^m \right] \alpha_j^3 \right. \\ &\quad \left. \left[ \sum_{k=0}^{m-1} \left( 1 - \frac{\alpha_j \mu}{4} \right)^k \right] \left[ \frac{Lm}{2} \left( 1 + \frac{240\alpha_j^2 \rho_w^2 L^3}{\mu(1-\rho_w^2)^2} \right) + \frac{240\rho_w^2 L^2}{\mu(1-\rho_w^2)^2} \right] \right\} \\ &\leq \prod_{j=0}^{t-1} \left( 1 - \frac{\alpha_j \mu}{4} \right)^m H_0 + \sum_{j=0}^{t-1} \left\{ \left[ \prod_{q=j+1}^{t-1} \left( 1 - \frac{\alpha_q \mu}{4} \right)^m \right] \alpha_j^3 \right. \\ &\quad \left. \left[ \sum_{k=0}^{m-1} \left( 1 - \frac{\alpha_j \mu}{4} \right)^k \right] \left( mL + \frac{240\rho_w^2 L^2}{\mu(1-\rho_w^2)^2} \right) \sigma_*^2 \right\} \quad (45)\end{aligned}$$

The last inequality holds for  $\alpha_j^2 \leq \frac{(1-\rho_w^2)^2 \mu}{240\rho_w^2 L^3}$  which is necessary for  $\alpha_j \leq \frac{(1-\rho_w^2)\mu}{8\sqrt{30}L^2}$ . Let  $\alpha_t = \alpha$  in (45). We obtain

$$\begin{aligned}H_t &\leq \left( 1 - \frac{\alpha \mu}{4} \right)^{mt} H_0 + \sum_{j=0}^{t-1} \left\{ \left[ \left( 1 - \frac{\alpha \mu}{4} \right)^{m(t-1-j)} \right] \right. \\ &\quad \left. \alpha^3 \left[ \sum_{k=0}^{m-1} \left( 1 - \frac{\alpha \mu}{4} \right)^k \right] \left( mL + \frac{240\rho_w^2 L^2}{\mu(1-\rho_w^2)^2} \right) \sigma_*^2 \right\} \\ &= \left( 1 - \frac{\alpha \mu}{4} \right)^{mt} H_0 \\ &\quad + \sum_{j=0}^{t-1} \sum_{k=0}^{m-1} \left[ \left( 1 - \frac{\alpha \mu}{4} \right)^{m(t-1-j)+k} \alpha^3 \right] \left( mL + \frac{240\rho_w^2 L^2}{\mu(1-\rho_w^2)^2} \right) \sigma_*^2 \\ &\leq \left( 1 - \frac{\alpha \mu}{4} \right)^{mt} H_0 + \frac{4\alpha^2}{\mu} \left( mL + \frac{240\rho_w^2 L^2}{\mu(1-\rho_w^2)^2} \right) \sigma_*^2. \quad (46)\end{aligned}$$

Substitute  $\alpha_t = \frac{\theta}{m\mu(t+K)}$  into (45), we obtain

$$\begin{aligned}H_t &\leq \prod_{j=0}^{t-1} \left( 1 - \frac{\theta}{4m(j+K)} \right)^m H_0 \\ &\quad + \sum_{j=0}^{t-1} \left\{ \left[ \prod_{q=j+1}^{t-1} \left( 1 - \frac{\theta}{4m(q+K)} \right)^m \right] \frac{1}{(j+K)^3} \right. \\ &\quad \left. \left[ \sum_{k=0}^{m-1} \left( 1 - \frac{\theta}{4m(j+K)} \right)^k \right] \left( mL + \frac{240\rho_w^2 L^2}{\mu(1-\rho_w^2)^2} \right) \frac{\theta^3 \sigma_*^2}{m^3 \mu^3} \right\} \\ &\leq \left( \frac{K}{t+K} \right)^{\frac{\theta}{4}} H_0 + \left( mL + \frac{240\rho_w^2 L^2}{\mu(1-\rho_w^2)^2} \right) \frac{\theta^3 \sigma_*^2}{m^3 \mu^3 (t+K)^{\theta/4}} \\ &\quad \cdot \sum_{j=0}^{t-1} \frac{(j+K+1)^{\theta/4} m}{(j+K)^3} \quad (47)\end{aligned}$$

$$\begin{aligned}&\leq \left( \frac{K}{t+K} \right)^{\frac{\theta}{4}} H_0 + \left[ \left( mL + \frac{240\rho_w^2 L^2}{\mu(1-\rho_w^2)^2} \right) \right. \\ &\quad \left. \cdot \frac{8\theta^3 \sigma_*^2}{m^2 \mu^3 (\theta-8)} \frac{1}{(t+K)^2} \right], \quad (48)\end{aligned}$$

where (47) holds for Lemma 4 by letting  $K \geq \frac{\theta}{2m}$  and  $\sum_{k=0}^{m-1} \left( 1 - \frac{\theta}{4m(j+K)} \right)^k \leq m$ . (48) holds because when  $K \geq \frac{\theta}{2} \geq \frac{\theta}{2m}$ ,

$$\left( \frac{j+K+1}{j+K} \right)^{\frac{\theta}{4}} \leq \left( 1 + \frac{1}{K} \right)^{\frac{\theta}{4}} \leq \left( 1 + \frac{2}{\theta} \right)^{\frac{\theta}{4}} \leq \exp \left( \frac{1}{2} \right) \leq 2,$$

and when  $\theta > 12$ ,

$$\sum_{j=0}^{t-1} (j+K)^{\theta/4-3} \leq \int_0^t (x+K)^{\theta/4-3} dx \leq \frac{4}{\theta-8} (t+K)^{\theta/4-2}.$$

□

## D. Proof of Lemma 10

*Proof.* Lemma 9 provides two upper bounds in the form of  $H_t \leq \mathcal{H}(\alpha_t)$  for some  $\mathcal{H}(\alpha_t)$  depending on the choice of the stepsize policy. Applying the upper bounds to (15) in Lemma 8 and invoking Lemma 6, we obtain

$$\begin{aligned}H_t^\ell &\leq \left( 1 - \frac{\alpha_t \mu}{4} \right)^\ell \mathcal{H}(\alpha_t) + 2 \left[ \frac{\alpha_t^3 L m \sigma_*^2}{4} \left( 1 + \frac{240\alpha_t^2 \rho_w^2 L^3}{\mu(1-\rho_w^2)^2} \right) \right. \\ &\quad \left. + \frac{120\alpha_t^3 \rho_w^2 L^2}{\mu(1-\rho_w^2)^2} \sigma_*^2 \right] \frac{4}{\alpha_t \mu}. \quad (49)\end{aligned}$$

If we use diminishing stepsizes  $\alpha_t = \frac{\theta}{m\mu(t+K)}$ , relation (49) and Lemma 9 yield

$$\begin{aligned}H_t^\ell &\leq \left( \frac{K}{t+K} \right)^{\frac{\theta}{4}} H_0 + \frac{4\theta^2 L \sigma_*^2}{m^2 \mu^3} \left( m + \frac{240\rho_w^2 L}{\mu(1-\rho_w^2)^2} \right) \frac{1}{(t+K)^2} \\ &\quad + \left( mL + \frac{240\rho_w^2 L^2}{\mu(1-\rho_w^2)^2} \right) \frac{8\theta^3 \sigma_*^2}{m^2 \mu^3 (\theta-8)} \frac{1}{(t+K)^2}.\end{aligned}$$

If we use a constant stepsize  $\alpha_t = \alpha$ , then (49) and Lemma 6 lead to

$$\begin{aligned}H_t^\ell &\leq \left( 1 - \frac{\alpha \mu}{4} \right)^{mt} H_0 + \frac{4\alpha^2}{\mu} \left( mL + \frac{240\rho_w^2 L^2}{\mu(1-\rho_w^2)^2} \right) \sigma_*^2 \\ &\quad + \frac{4\alpha^2 L}{\mu} \left( m + \frac{240\rho_w^2 L}{\mu(1-\rho_w^2)^2} \right) \sigma_*^2.\end{aligned}$$

Rearranging the terms and noting that  $\theta > 12$ , we obtain the desired result.  $\square$

### E. Proof of Lemma 12

*Proof.* Apply Lemma 11 into Lemma 5 and note  $\alpha_t \leq \frac{1}{\mu}$ , we have

$$\begin{aligned} \mathbb{E} \left[ \|\bar{x}_t^{\ell+1} - \bar{x}_*^{\ell+1}\|^2 \right] &\leq (1 - \frac{\alpha_t \mu}{2}) \mathbb{E} \left[ \|\bar{x}_t^\ell - \bar{x}_*^\ell\|^2 \right] \\ &\quad + 2\alpha_t \sigma_{\text{shuffle}}^2 + \frac{2\alpha_t L^2}{n} \left( \frac{1}{\mu} + \alpha_t \right) \left\{ \left( \frac{1 + \rho_w^2}{2} \right)^{mt} \right. \\ &\quad \cdot \|\mathbf{x}_0^0 - \mathbf{1}(\bar{x}_0^0)^\top\|^2 + \frac{4\hat{X}_1}{(1 - \rho_w^2)^2} \alpha_t^2 \left. \right\} \end{aligned}$$

Invoke relation (38) and Lemma 6, we obtain

$$\begin{aligned} \mathbb{E} \left[ \|\bar{x}_{t+1}^0 - x^*\|^2 \right] &\leq (1 - \frac{\alpha_t \mu}{2})^m \mathbb{E} \left[ \|\bar{x}_t^0 - x^*\|^2 \right] \\ &\quad + \frac{\alpha_t^3 L m \sigma_*^2}{2} \left[ \sum_{k=0}^{m-1} \left( 1 - \frac{\alpha_t \mu}{2} \right)^k \right] + \frac{4\alpha_t L^2}{n \mu^2} \left\{ \left( \frac{1 + \rho_w^2}{2} \right)^{mt} \right. \\ &\quad \cdot \|\mathbf{x}_0^0 - \mathbf{1}(\bar{x}_0^0)^\top\|^2 + \frac{4\hat{X}_1}{(1 - \rho_w^2)^2} \alpha_t^2 \left. \right\} \left[ \sum_{k=0}^{m-1} \left( 1 - \frac{\alpha_t \mu}{2} \right)^k \right] \end{aligned}$$

Unroll the above, we have

$$\begin{aligned} \mathbb{E} \left[ \|\bar{x}_t^0 - x^*\|^2 \right] &\leq \prod_{j=0}^{t-1} \left( 1 - \frac{\alpha_j \mu}{2} \right)^m \|\bar{x}_0^0 - x^*\|^2 \\ &\quad + \frac{m L \sigma_*^2}{2} \sum_{j=0}^{t-1} \left\{ \left[ \prod_{q=j+1}^{t-1} \left( 1 - \frac{\alpha_q \mu}{2} \right)^m \right] \alpha_j^3 \left[ \sum_{k=0}^{m-1} \left( 1 - \frac{\alpha_j \mu}{2} \right)^k \right] \right\} \\ &\quad + \sum_{j=0}^{t-1} \left\{ \left[ \prod_{q=j+1}^{t-1} \left( 1 - \frac{\alpha_q \mu}{2} \right)^m \right] \frac{4\alpha_j L^2}{n \mu^2} \left[ \left( \frac{1 + \rho_w^2}{2} \right)^{mj} \right. \right. \\ &\quad \cdot \|\mathbf{x}_0^0 - \mathbf{1}(\bar{x}_0^0)^\top\|^2 + \frac{4\hat{X}_1}{(1 - \rho_w^2)^2} \alpha_j^2 \left. \left. \right] \left[ \sum_{k=0}^{m-1} \left( 1 - \frac{\alpha_j \mu}{2} \right)^k \right] \right\} \end{aligned}$$

Similar to those in deriving Lemma 9 and by  $K \geq \theta$ , we obtain

$$\begin{aligned} \mathbb{E} \left[ \|\bar{x}_t^0 - x^*\|^2 \right] &\leq \left( \frac{K}{t+K} \right)^{\frac{\theta}{2}} \|\bar{x}_0^0 - x^*\|^2 \\ &\quad + \frac{2\theta^3 L \sigma_*^2}{m \mu^3 (\theta - 4)} \frac{1}{(t+K)^2} + \frac{96\theta^3 L^2 \hat{X}_1}{n m^2 \mu^5 (1 - \rho_w^2)^2 (\theta - 4)} \frac{1}{(t+K)^2} \\ &\quad + \left( \frac{K}{t+K} \right)^{\frac{\theta}{2}} \frac{96L^2}{n \mu^3 (1 - \rho_w^2)} \|\mathbf{x}_0^0 - \mathbf{1}(\bar{x}_0^0)^\top\|^2. \end{aligned}$$

The last term is because  $(t+K)^{\theta/2-1} q_0^t$  is decreasing in  $t$  with  $q_0 := \left( \frac{1+\rho_w^2}{2} \right)^m$ , then

$$\begin{aligned} &\frac{1}{\ln q_0} d \left( (t+K)^{\frac{\theta}{2}-1} q_0^t \right) \\ &= \frac{1}{\ln q_0} \left( \frac{\theta}{2} - 1 \right) (t+K)^{\frac{\theta}{2}-2} q_0^t dt + (t+K)^{\frac{\theta}{2}-1} q_0^t dt \\ &\geq \frac{1}{2} (t+K)^{\frac{\theta}{2}-1} q_0^t dt. \end{aligned}$$

Thus,

$$\begin{aligned} \sum_{j=0}^{t-1} (j+K)^{\frac{\theta}{2}-1} q_0^j &\leq \int_0^\infty (t+K)^{\theta/2-1} q_0^t dt \\ &\leq \frac{2}{\ln q_0} \int_K^\infty \frac{d \left( (t+K)^{\frac{\theta}{2}-1} q_0^{t-K} \right)}{dt} = -\frac{2K^{\frac{\theta}{2}-1}}{\ln q_0} \leq \frac{4K^{\frac{\theta}{2}-1}}{m(1 - \rho_w^2)}. \end{aligned}$$

$\square$

### F. Proof of Corollary 1

*Proof.* Note for  $\alpha$  satisfying (14),

$$H_0 = \mathcal{O} \left( \frac{n \|\bar{x}_0^0 - x^*\|^2 + \|\mathbf{x}_0^0 - \mathbf{1}(\bar{x}_0^0)^\top\|^2}{n} \right).$$

Rearrange the result in Theorem 2 and notice  $(1-x) \leq \exp(-x)$ . We obtain

$$\begin{aligned} \frac{1}{n} \sum_{i=1}^n \mathbb{E} \left[ \|x_{i,T}^0 - x^*\|^2 \right] &\leq \exp \left( -\frac{\alpha \mu m T}{4} \right) H_0 + \frac{4\alpha^2 m L \sigma_*^2}{\mu} \\ &\quad + \frac{4\hat{X}_1}{n(1 - \rho_w^2)^2} \alpha^2 + \frac{960 \rho_w^2 L^2 \sigma_*^2}{\mu^2 (1 - \rho_w^2)^2} \alpha^2 \\ &\quad + \exp \left( -\frac{1 - \rho_w^2}{2} m T \right) \frac{\|\mathbf{x}_0^0 - \mathbf{1}(\bar{x}_0^0)^\top\|^2}{n}. \end{aligned} \quad (50)$$

Denoting the stepsize satisfying (14) as  $\bar{\alpha}$  and using  $\tilde{\mathcal{O}}(\cdot)$  to hide the logarithm factors, it is sufficient to discuss the following two cases:

**Case I:** If  $\alpha = \frac{4}{LmT} \log \frac{H_0 \mu^2 m T^2}{\kappa \sigma_*^2} \leq \bar{\alpha}$ , then we substitute such an  $\alpha \leq \frac{4}{\mu m T} \log \frac{H_0 \mu^2 m T^2}{\kappa \sigma_*^2}$  into (50) and get

$$\begin{aligned} \frac{1}{n} \sum_{i=1}^n \mathbb{E} \left[ \|x_{i,T}^0 - x^*\|^2 \right] &= \tilde{\mathcal{O}} \left( \frac{\kappa \sigma_*^2}{\mu^2 m T^2} \right) \\ &\quad + \exp \left( -\frac{1 - \rho_w^2}{2} m T \right) \frac{\|\mathbf{x}_0^0 - \mathbf{1}(\bar{x}_0^0)^\top\|^2}{n} \\ &\quad + \tilde{\mathcal{O}} \left( \frac{\hat{X}_1}{L^2 n m^2 (1 - \rho_w^2)^2 T^2} \right) + \tilde{\mathcal{O}} \left( \frac{\sigma_*^2}{\mu^2 (1 - \rho_w^2)^2 m^2 T^2} \right). \end{aligned}$$

**Case II:** If  $\bar{\alpha} < \frac{4}{LmT} \log \frac{H_0 \mu^2 m T^2}{\kappa \sigma_*^2} \leq \frac{4}{\mu m T} \log \frac{H_0 \mu^2 m T^2}{\kappa \sigma_*^2}$ , we substitute  $\bar{\alpha}$  into (50) and obtain,

$$\begin{aligned} \frac{1}{n} \sum_{i=1}^n \mathbb{E} \left[ \|x_{i,T}^0 - x^*\|^2 \right] &= \exp \left( -\frac{\bar{\alpha} \mu m T}{4} \right) H_0 \\ &\quad + \exp \left( -\frac{1 - \rho_w^2}{2} m T \right) \frac{\|\mathbf{x}_0^0 - \mathbf{1}(\bar{x}_0^0)^\top\|^2}{n} + \tilde{\mathcal{O}} \left( \frac{\kappa \sigma_*^2}{\mu^2 m T^2} \right) \\ &\quad + \tilde{\mathcal{O}} \left( \frac{\hat{X}_1}{n m^2 L^2 (1 - \rho_w^2)^2 T^2} \right) + \tilde{\mathcal{O}} \left( \frac{\sigma_*^2}{(1 - \rho_w^2)^2 \mu^2 m^2 T^2} \right). \end{aligned}$$

We finish our proof by noting that

$$\hat{X}_1 = \mathcal{O} \left( \frac{(n \|\bar{x}_0^0 - x^*\|^2 + \|\mathbf{x}_0^0 - \mathbf{1}(\bar{x}_0^0)^\top\|^2) L^2}{1 - \rho_w^2} + \frac{m n \sigma_*^2}{1 - \rho_w^2} \right).$$

$\square$

## APPENDIX C PROOFS FOR THE NONCONVEX CASE

### A. Proof of Lemma 3

*Proof.* The proof is similar to [23, Proposition 2], we present it here for completeness. By Assumption 3, we have

$$\|\nabla f_{i,\ell}(x)\| \leq 2L(f_{i,\ell}(x) - \bar{f}_{i,\ell}), \quad \forall x \in \mathbb{R}^p, \quad i, \ell.$$

Therefore,

$$\begin{aligned} \frac{1}{mn} \sum_{i=1}^n \sum_{\ell=1}^m \|\nabla f_{i,\ell}(x) - \nabla f(x)\|^2 &\leq \frac{1}{mn} \sum_{i=1}^n \sum_{\ell=1}^m \|\nabla f_{i,\ell}(x)\|^2 \\ &\leq \frac{2L}{mn} \sum_{i=1}^n \sum_{\ell=1}^m (f_{i,\ell}(x) - \bar{f}_{i,\ell}) \\ &= 2L(f(x) - \bar{f}) + 2L \left( \bar{f} - \frac{1}{mn} \sum_{i=1}^n \sum_{\ell=1}^m \bar{f}_{i,\ell} \right). \end{aligned}$$

$$\text{We have } A = \frac{2L}{mn} > 0 \quad \text{and} \quad B^2 = 2L \left( \bar{f} - \frac{1}{mn} \sum_{i=1}^n \sum_{\ell=1}^m \bar{f}_{i,\ell} \right) \geq 0. \quad \square$$

### B. Proof of Lemma 13

*Proof.* By  $L$ -smoothness of the objective function  $f$ , we obtain

$$\begin{aligned} f(\bar{x}_{t+1}^0) &\leq f(\bar{x}_t^0) - \langle \nabla f(\bar{x}_t^0), \bar{x}_t^0 - \bar{x}_{t+1}^0 \rangle + \frac{L}{2} \|\bar{x}_{t+1}^0 - \bar{x}_t^0\|^2 \\ &= f(\bar{x}_t^0) - \alpha m \left\langle \nabla f(\bar{x}_t^0), \frac{1}{mn} \sum_{\ell=0}^{m-1} \sum_{i=1}^n \nabla f_{i,\pi_\ell^i}(x_{i,t}^\ell) \right\rangle \\ &\quad + \frac{L}{2} \left\| \frac{\alpha}{n} \sum_{\ell=0}^{m-1} \sum_{i=1}^n \nabla f_{i,\pi_\ell^i}(x_{i,t}^\ell) \right\|^2 \\ &= f(\bar{x}_t^0) - \frac{\alpha m}{2} \|\nabla f(\bar{x}_t^0)\|^2 \\ &\quad - \frac{\alpha m}{2} (1 - \alpha m L) \left\| \frac{1}{mn} \sum_{\ell=0}^{m-1} \sum_{i=1}^n \nabla f_{i,\pi_\ell^i}(x_{i,t}^\ell) \right\|^2 \\ &\quad + \frac{\alpha m}{2} \left\| \frac{1}{mn} \sum_{\ell=0}^{m-1} \sum_{i=1}^n \nabla f_{i,\pi_\ell^i}(x_{i,t}^\ell) - \nabla f(\bar{x}_t^0) \right\|^2, \end{aligned} \quad (51)$$

where we invoke  $\langle a, b \rangle = (\|a\|^2 + \|b\|^2 - \|a - b\|^2)/2$ .

Then, utilizing  $L$ -smoothness of each component function yields

$$\begin{aligned} &\left\| \frac{1}{mn} \sum_{\ell=0}^{m-1} \sum_{i=1}^n \nabla f_{i,\pi_\ell^i}(x_{i,t}^\ell) - \nabla f(\bar{x}_t^0) \right\|^2 \\ &\leq \frac{L^2}{mn} \sum_{\ell=0}^{m-1} \sum_{i=1}^n \|x_{i,t}^\ell - \bar{x}_t^0\|^2 \\ &\leq \frac{2L^2}{mn} \sum_{\ell=0}^{m-1} \|\mathbf{x}_t^\ell - \mathbf{1}(\bar{x}_t^\ell)^\top\|^2 + \frac{2L^2}{m} \sum_{\ell=0}^{m-1} \|\bar{x}_t^\ell - \bar{x}_t^0\|^2. \end{aligned} \quad (52)$$

Inserting (52) into (51) and using the condition  $\alpha \leq \frac{1}{mL}$  finish the proof.  $\square$

### C. Proof of Lemma 14

*Proof.* By the update (4) and Young's inequality for  $q = \frac{1+\rho_w^2}{2\rho_w^2}$ , we have

$$\begin{aligned} \|\mathbf{x}_t^{\ell+1} - \mathbf{1}(\bar{x}_t^{\ell+1})^\top\|^2 &\leq \left\| \left( W - \frac{\mathbf{1}\mathbf{1}^\top}{n} \right) (\mathbf{x}_t^\ell - \alpha \nabla F_{\pi_\ell}(\mathbf{x}_t^\ell)) \right\|^2 \\ &\leq \frac{1+\rho_w^2}{2} \|\mathbf{x}_t^\ell - \mathbf{1}(\bar{x}_t^\ell)^\top\|^2 + \frac{2\alpha^2}{1-\rho_w^2} \|\nabla F_{\pi_\ell}(\mathbf{x}_t^\ell)\|^2. \end{aligned} \quad (53)$$

It follows that

$$\begin{aligned} \sum_{\ell=0}^{m-1} \|\mathbf{x}_t^\ell - \mathbf{1}(\bar{x}_t^\ell)^\top\|^2 &\leq \frac{2}{1-\rho_w^2} \|\mathbf{x}_t^0 - \mathbf{1}(\bar{x}_t^0)^\top\|^2 \\ &\quad + \frac{2\alpha^2}{1-\rho_w^2} \sum_{\ell=0}^{m-1} \sum_{j=0}^{\ell-1} \left( \frac{1+\rho_w^2}{2} \right)^{\ell-j-1} \sum_{i=1}^n \|\nabla f_{i,\pi_j^i}(x_{i,t}^j)\|^2. \end{aligned} \quad (54)$$

Next consider the last term in (54). We have

$$\begin{aligned} &\frac{1}{3} \sum_{\ell=0}^{m-1} \sum_{j=0}^{\ell-1} \left( \frac{1+\rho_w^2}{2} \right)^{\ell-j-1} \sum_{i=1}^n \|\nabla f_{i,\pi_j^i}(x_{i,t}^j)\|^2 \\ &\leq \sum_{\ell=0}^{m-1} \sum_{j=0}^{\ell-1} \left( \frac{1+\rho_w^2}{2} \right)^{\ell-j-1} \sum_{i=1}^n \left\{ \|\nabla f_{i,\pi_j^i}(x_{i,t}^j) - \nabla f_{i,\pi_j^i}(\bar{x}_t^0)\|^2 \right. \\ &\quad \left. + \|\nabla f_{i,\pi_j^i}(\bar{x}_t^0) - \nabla f(\bar{x}_t^0)\|^2 + \|\nabla f(\bar{x}_t^0)\|^2 \right\} \\ &\leq \sum_{\ell=0}^{m-1} \sum_{j=0}^{\ell-1} \left( \frac{1+\rho_w^2}{2} \right)^{\ell-j-1} \sum_{i=1}^n \left\{ L^2 \|x_{i,t}^j - \bar{x}_t^0\|^2 \right. \\ &\quad \left. + \|\nabla f_{i,\pi_j^i}(\bar{x}_t^0) - \nabla f(\bar{x}_t^0)\|^2 + \|\nabla f(\bar{x}_t^0)\|^2 \right\} \end{aligned} \quad (55)$$

$$\begin{aligned} &\leq \frac{2L^2}{1-\rho_w^2} \sum_{\ell=0}^{m-1} \sum_{i=1}^n \|x_{i,t}^\ell - \bar{x}_t^0\|^2 + \frac{2mn}{1-\rho_w^2} \|\nabla f(\bar{x}_t^0)\|^2 \\ &\quad + \frac{2m^2n}{1-\rho_w^2} [2A(f(\bar{x}_t^0) - \bar{f}) + B^2], \end{aligned} \quad (56)$$

where (55) comes from Assumption 3, and (56) holds by Lemma 3. Combining (52), (54) and (56) leads to

$$\begin{aligned} \sum_{\ell=0}^{m-1} \|\mathbf{x}_t^\ell - \mathbf{1}(\bar{x}_t^\ell)^\top\|^2 &\leq \frac{2}{1-\rho_w^2} \|\mathbf{x}_t^0 - \mathbf{1}(\bar{x}_t^0)^\top\|^2 + \frac{12B^2\alpha^2m^2n}{(1-\rho_w^2)^2} \\ &\quad + \frac{12mn\alpha^2}{(1-\rho_w^2)^2} \|\nabla f(\bar{x}_t^0)\|^2 + \frac{24\alpha^2nL^2}{(1-\rho_w^2)^2} \sum_{\ell=0}^{m-1} \|\bar{x}_t^\ell - \bar{x}_t^0\|^2 \\ &\quad + \frac{24\alpha^2L^2}{(1-\rho_w^2)^2} \sum_{\ell=0}^{m-1} \|\mathbf{x}_t^\ell - \mathbf{1}(\bar{x}_t^\ell)^\top\|^2 \\ &\quad + \frac{24A\alpha^2m^2n}{(1-\rho_w^2)^2} (f(\bar{x}_t^0) - \bar{f}). \end{aligned}$$

Similar to (56), we have

$$\begin{aligned}
\sum_{\ell=0}^{m-1} \|\bar{x}_t^\ell - \bar{x}_t^0\|^2 &= m^2 \alpha^2 \sum_{\ell=0}^{m-1} \left\| \frac{1}{mn} \sum_{j=0}^{\ell-1} \sum_{i=1}^n \nabla f_{i,\pi_j^i}(x_{i,t}^j) \right\|^2 \\
&\leq \frac{m\alpha^2}{n} \sum_{\ell=0}^{m-1} \sum_{j=0}^{\ell-1} \sum_{i=1}^n \|\nabla f_{i,\pi_j^i}(x_{i,t}^j)\|^2 \\
&\leq \frac{6m^2\alpha^2L^2}{n} \sum_{\ell=0}^{m-1} \|\mathbf{x}_t^\ell - \mathbf{1}(\bar{x}_t^\ell)^\top\|^2 + 6m^2\alpha^2L^2 \sum_{\ell=0}^{m-1} \|\bar{x}_t^\ell - \bar{x}_t^0\|^2 \\
&\quad + 3m^3\alpha^2 [2A(f(\bar{x}_t^0) - \bar{f}) + B^2] + 3m^3\alpha^2 \|\nabla f(\bar{x}_t^0)\|^2. \tag{57}
\end{aligned}$$

Since  $\mathcal{L}_t = \frac{1}{n} \sum_{\ell=0}^{m-1} \|\mathbf{x}_t^\ell - \mathbf{1}(\bar{x}_t^\ell)^\top\|^2 + \sum_{\ell=0}^{m-1} \|\bar{x}_t^\ell - \bar{x}_t^0\|^2$ , we have

$$\begin{aligned}
\left(1 - 6m^2\alpha^2L^2 - \frac{24\alpha^2L^2}{(1-\rho_w^2)^2}\right) \mathcal{L}_t &\leq \frac{2}{n(1-\rho_w^2)} \|\mathbf{x}_t^0 - \mathbf{1}(\bar{x}_t^0)^\top\|^2 \\
&\quad + \frac{3m^2\alpha^2B^2(m+4)}{(1-\rho_w^2)^2} + \frac{3\alpha^2m(4+m^2)}{(1-\rho_w^2)^2} \|\nabla f(\bar{x}_t^0)\|^2 \\
&\quad + \frac{6m^2\alpha^2A(4+m)}{(1-\rho_w^2)} (f(\bar{x}_t^0) - \bar{f}).
\end{aligned}$$

Let

$$\alpha \leq \min \left\{ \frac{1}{2\sqrt{6mL}}, \frac{1-\rho_w^2}{4\sqrt{6L}} \right\}.$$

We obtain the desired result for  $\mathcal{L}_t$ . Then, from (53), we have

$$\begin{aligned}
\|\mathbf{x}_{t+1}^0 - \mathbf{1}(\bar{x}_{t+1}^0)^\top\|^2 &= \|\mathbf{x}_t^m - \mathbf{1}(\bar{x}_t^m)^\top\|^2 \\
&\leq \left(\frac{1+\rho_w^2}{2}\right)^m \|\mathbf{x}_t^0 - \mathbf{1}(\bar{x}_t^0)^\top\|^2 \\
&\quad + \frac{2\alpha^2}{1-\rho_w^2} \sum_{j=0}^{m-1} \left(\frac{1+\rho_w^2}{2}\right)^{m-j-1} \|\nabla F_{\pi_j}(\mathbf{x}_t^j)\|^2 \\
&\leq \left(\frac{1+\rho_w^2}{2}\right)^m \|\mathbf{x}_t^0 - \mathbf{1}(\bar{x}_t^0)^\top\|^2 + \frac{2\alpha^2}{1-\rho_w^2} \sum_{j=0}^{m-1} \|\nabla F_{\pi_j}(\mathbf{x}_t^j)\|^2 \\
&\leq \left(\frac{1+\rho_w^2}{2}\right)^m \|\mathbf{x}_t^0 - \mathbf{1}(\bar{x}_t^0)^\top\|^2 + \frac{12\alpha^2L^2}{1-\rho_w^2} \sum_{j=0}^{m-1} \|\mathbf{x}_t^j - \mathbf{1}(\bar{x}_t^j)^\top\|^2 \\
&\quad + \frac{12\alpha^2L^2n}{1-\rho_w^2} \sum_{j=0}^{m-1} \|\bar{x}_t^j - \bar{x}_t^0\|^2 + \frac{6\alpha^2mn}{1-\rho_w^2} \|\nabla f(\bar{x}_t^0)\|^2 \\
&\quad + \frac{6\alpha^2mn}{1-\rho_w^2} [2A(f(\bar{x}_t^0) - \bar{f}) + B^2]. \tag{58}
\end{aligned}$$

□

#### D. Proof of Lemma 15

*Proof.* Substituting  $\mathcal{L}_t$  into Lemma 13 yields

$$\begin{aligned}
f(\bar{x}_{t+1}^0) &\leq f(\bar{x}_t^0) - \frac{m\alpha}{2} \|\nabla f(\bar{x}_t^0)\|^2 + \alpha L^2 \mathcal{L}_t \\
&\leq f(\bar{x}_t^0) - \frac{m\alpha}{2} \|\nabla f(\bar{x}_t^0)\|^2 + \frac{4\alpha L^2}{n(1-\rho_w^2)} \|\mathbf{x}_t^0 - \mathbf{1}(\bar{x}_t^0)^\top\|^2 \\
&\quad + \frac{6m^2\alpha^3B^2(m+4)L^2}{(1-\rho_w^2)^2} + \frac{6\alpha^3m(4+m^2)L^2}{(1-\rho_w^2)^2} \|\nabla f(\bar{x}_t^0)\|^2 \\
&\quad + \frac{12m^2\alpha^3L^2A(4+m)}{(1-\rho_w^2)} (f(\bar{x}_t^0) - \bar{f}). \tag{59}
\end{aligned}$$

Combining the two recursions in Lemma 14 and letting  $\alpha \leq \left(\frac{(1-\rho_w^2)^3}{192L^2}\right)^{1/2}$ , we have

$$\begin{aligned}
\|\mathbf{x}_{t+1}^0 - \mathbf{1}(\bar{x}_{t+1}^0)^\top\|^2 &\leq \frac{3+\rho_w^2}{4} \|\mathbf{x}_t^0 - \mathbf{1}(\bar{x}_t^0)^\top\|^2 \\
&\quad + \frac{6\alpha^2mnB^2}{1-\rho_w^2} \left(1 + \frac{12\alpha^2L^2m(m+4)}{(1-\rho_w^2)^2}\right) \\
&\quad + \frac{6\alpha^2mn}{1-\rho_w^2} \left(1 + \frac{12\alpha^2L^2(m^2+4)}{(1-\rho_w^2)^2}\right) \|\nabla f(\bar{x}_t^0)\|^2 \\
&\quad + \frac{12A\alpha^2mn}{1-\rho_w^2} \left(1 + \frac{12\alpha^2L^2m(m+4)}{(1-\rho_w^2)^2}\right) (f(\bar{x}_t^0) - \bar{f}) \\
&\leq \frac{3+\rho_w^2}{4} \|\mathbf{x}_t^0 - \mathbf{1}(\bar{x}_t^0)^\top\|^2 + \frac{12\alpha^2mnB^2}{1-\rho_w^2} \\
&\quad + \frac{12\alpha^2mn}{1-\rho_w^2} \|\nabla f(\bar{x}_t^0)\|^2 + \frac{24A\alpha^2mn}{1-\rho_w^2} (f(\bar{x}_t^0) - \bar{f}), \tag{60}
\end{aligned}$$

where the last inequality holds by letting  $\alpha \leq \frac{1-\rho_w^2}{2\sqrt{3(m+2)L}}$ . Combining (59) and (60) yields

$$\begin{aligned}
f(\bar{x}_{t+1}^0) - \bar{f} &+ \frac{16\alpha L^2}{n(1-\rho_w^2)^2} \|\mathbf{x}_{t+1}^0 - \mathbf{1}(\bar{x}_{t+1}^0)^\top\|^2 \\
&\leq \left[1 + \frac{12m^2\alpha^3L^2A(4+m)}{(1-\rho_w^2)} + \frac{384A\alpha^3L^2m}{(1-\rho_w^2)^3}\right] (f(\bar{x}_t^0) - \bar{f}) \\
&\quad + \frac{16\alpha L^2}{n(1-\rho_w^2)^2} \|\mathbf{x}_t^0 - \mathbf{1}(\bar{x}_t^0)^\top\|^2 + \frac{6m\alpha^3L^2B^2[m(m+4)+32]}{(1-\rho_w^2)^3} \\
&\quad - \frac{m\alpha}{2} \left(1 - \frac{12\alpha^2(4+m^2)L^2}{(1-\rho_w^2)^2} - \frac{384\alpha^2L^2}{(1-\rho_w^2)^3}\right) \|\nabla f(\bar{x}_t^0)\|^2. \tag{61}
\end{aligned}$$

Since  $Q_t$  is defined as

$$Q_t := f(\bar{x}_t^0) - \bar{f} + \frac{16\alpha L^2}{n(1-\rho_w^2)^2} \|\mathbf{x}_t^0 - \mathbf{1}(\bar{x}_t^0)^\top\|^2,$$

relation (61) becomes

$$\begin{aligned}
Q_{t+1} &\leq \left[1 + \frac{12m^2\alpha^3L^2A(4+m)}{(1-\rho_w^2)} + \frac{384A\alpha^3L^2m}{(1-\rho_w^2)^3}\right] Q_t \\
&\quad - \frac{m\alpha}{4} \|\nabla f(\bar{x}_t^0)\|^2 + \frac{6m\alpha^3L^2B^2[m(m+4)+32]}{(1-\rho_w^2)^3}, \tag{62}
\end{aligned}$$

where we invoke  $\alpha \leq \min \left\{ \frac{1-\rho_w^2}{4\sqrt{3L(m+2)}}, \frac{(1-\rho_w^2)^{3/2}}{16\sqrt{6L}} \right\}$ . □
